# Supplementary material for: Prototypes are Balanced Units for Efficient and Effective Partially Relevant Video Retrieval
Source: arXiv:2504.13035 source file (2025-04-17)
Supplement: Supplementary file 1 [file 0_extended_related_work.tex]

\section{Extended Related Work}
In the literature on Text-Video Retrieval, single video moment retrieval and video corpus moment retrieval are other closely related research areas.

\subsection{Extended Text-Video Retrieval}
\noindent\textbf{Video moment retrieval} aims to localize partial moments in videos that corresponds to the text descriptions~\cite{anne2017localizing, gao2017tall, soldan2021vlg, mr1, mr2, mr3, mr4,liu2021context,zhang2019exploiting,zhang2019man, qddetr, eatr, univtg,unloc, momentdetr, umt}.
As it only requires pair-wise computation during inference time~(to search for the moment in paired video), video-query interactive designs are popularly employed~\cite{xiao2024bridging, cgdetr, trdetr}.

\noindent\textbf{Video corpus moment retrieval}~\cite{hou2024improving, zhang2021multi}, on the other hand, requires multiple videos to be considered at once, thus modality-interactive designs are rarely adopted.
Consequently, recent works consider a two-stage pipeline where video retrieval models are adopted to enable the video-query interactive designs~\cite{conquer,vcmr}.
We note that without the task of moment retrieval, video corpus moment retrieval becomes very similar to PRVR to retrieve a video that contains the referred content.

\subsection{Representation Learning}
From pretext tasks\cite{dosovitskiy2014discriminative, doersch2015unsupervised, noroozi2016unsupervised, mundhenk2018improvements, gidaris2018unsupervised, moon2022tailoring} to contrastive learning~\cite{chen2021exploring, he2020momentum, chen2020simple, caron2020unsupervised, tian2021understanding} and to mask generation~\cite{he2022masked, tong2022videomae, bachmann2022multimae}, representation learning has been through dramatic evolvement.
Among them, our objectives include contrastive learning and mask generation.
Contrastive learning, in particular, is widely used in retrieval tasks because its process of minimizing the distances between paired instances while maximizing those between unpaired ones naturally aligns with the goals of retrieval.
Mask generation, as explored in prior work~\cite{he2022masked}, is another technique that enhances the model's understanding of input data by requiring it to predict masked content. In this work, we adapt mask generation for the PRVR task in two key aspects: first, we use InfoNCE to align the mask generation task with the objectives of PRVR, and second, we generate masked text using only the retrieved prototype.
