# Supplementary material for: Prototypes are Balanced Units for Efficient and Effective Partially Relevant Video Retrieval
Source: arXiv:2504.13035 source file (2025-04-17)
Supplement: Supplementary file 2 [file 3_analysis_attention.tex]

\section{Further Analysis of Retrieved prototype}
\label{sec:sup_attention_analysis}
\begin{figure}[h!]
    \centering
    \includegraphics[width=0.48\textwidth]{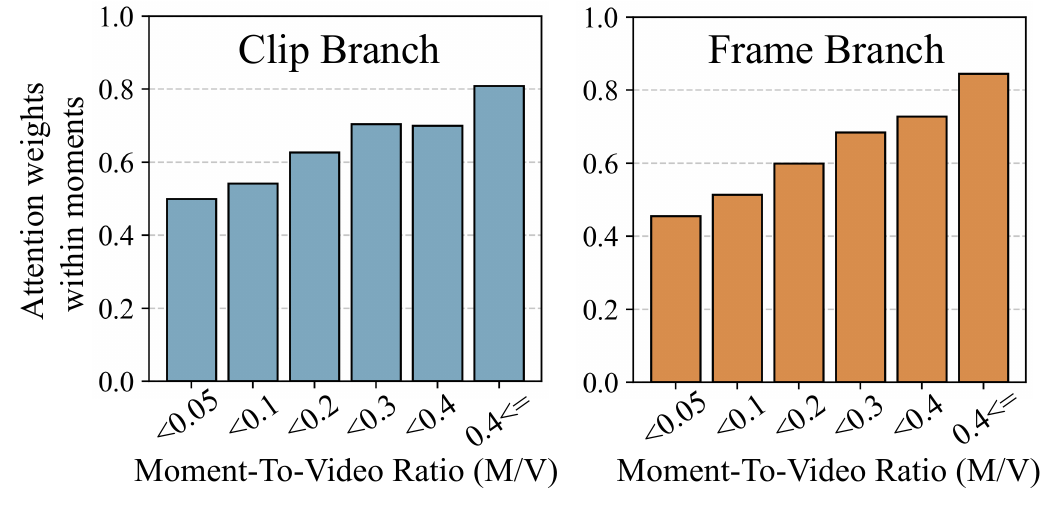}
    \caption{
    % Attendance on frames within moments for visual prototypes.
    % (\textit{Left}) We plot how much each prototype attends to the frames within moments in the order of the similarity to a given query.
    % The higher the similarity between the prototype and the text query, we observe the higher attendance on moment frames.
    Analysis of the magnitude of attendance on the moment frames of the retrieved prototypes $\hat{P}_*$, categorized by the Moment-To-Video ratio.
    }
    \label{fig:attention_qualitative_mtv}
\end{figure}

% \subsubsection{Per-instance Prototypes: Where do the retrieved prototypes focus?}
% In this subsection, we analyze whether the prototypes encode the specified semantics.
% Particularly, we visualize the magnitude of prototypes' attention weights on the in-moment frames including the text-relevant contexts.
% Note that the temporal margin is added to moment boundaries, \textit{i.e.}, start and end indices of moments are formed as [st - tm, ed + tm] following \cite{zhao2017temporal, lin2018bsn}, since understanding the nearby context is also important to comprehend the moments~(tm is set to about 1.5 seconds).

% In Fig.~\ref{fig:attention_qualitative_rank}, we plot the attention magnitude within the moment frames of each prototype in the order of the similarity between each prototype and the text description.
% Specifically, we observe that the retrieval score~(similarity) is highly correlated with the degree of attendance on in-moment frames.
% This validates the contextual understanding capability of our prototypical learning framework.

% Besides, the average attention weights within moments are not near the maximum attention weight~(1).
% We attribute this phenomenon to two primary reasons; (1) the specified moments in PRVR tasks are usually very short and (2) prototypes are aggregated without the indications of the textual descriptions' abstraction level and temporal spans of corresponding moments within the videos.
% our framework's proficiency in identifying relevant video segments in partially relevant video retrieval scenarios.
In Fig.~6 in the manuscript, we observed a strong correlation between the attention magnitude within moment frames and the retrieval score~(similarity).
This study further explores the relationship between attention weights and the retrieval score under varying Moment-To-Video ratios.
Fig.~\ref{fig:attention_qualitative_mtv} illustrates the distribution of attention weights within moments across different moment-to-video ratios.
As observed, the attention weights within moments of retrieved prototypes~(y-axis) significantly exceed the corresponding Moment-To-Video ratios~(x-axis).
% Notably, we highlight the substantial attention magnitude when the moment-to-video ratio is below 0.05; although the moment only possesses 5\% of the given video which is difficult to be captured, our proposed method effectively captures the moment and exhibit high attention magnitude~(around 0.5).
Notably, we observe a substantial attention magnitude when the moment-to-video ratio is below 0.05. 
Although the moments typically comprise less than 5\% of the entire video which indicates the challenge in detecting these moments, our proposed method effectively identifies the moment, demonstrating a high attention magnitude of approximately 0.5.
% Notably, we highlight the substantial attention magnitude~(around 0.5) within moments when the moment-to-video ratio is below 0.05, indicating that the moment is difficult to capture.
These results demonstrate our framework's proficiency in identifying relevant video segments within partially relevant video retrieval scenarios.
