# Supplementary material for: Prototypes are Balanced Units for Efficient and Effective Partially Relevant Video Retrieval
Source: arXiv:2504.13035 source file (2025-04-17)
Supplement: Supplementary file 3 [file 4_qualitative.tex]

\begin{figure*}[t!]
    \centering
    % \vspace{-0.3cm}
    \includegraphics[width=0.9\textwidth]{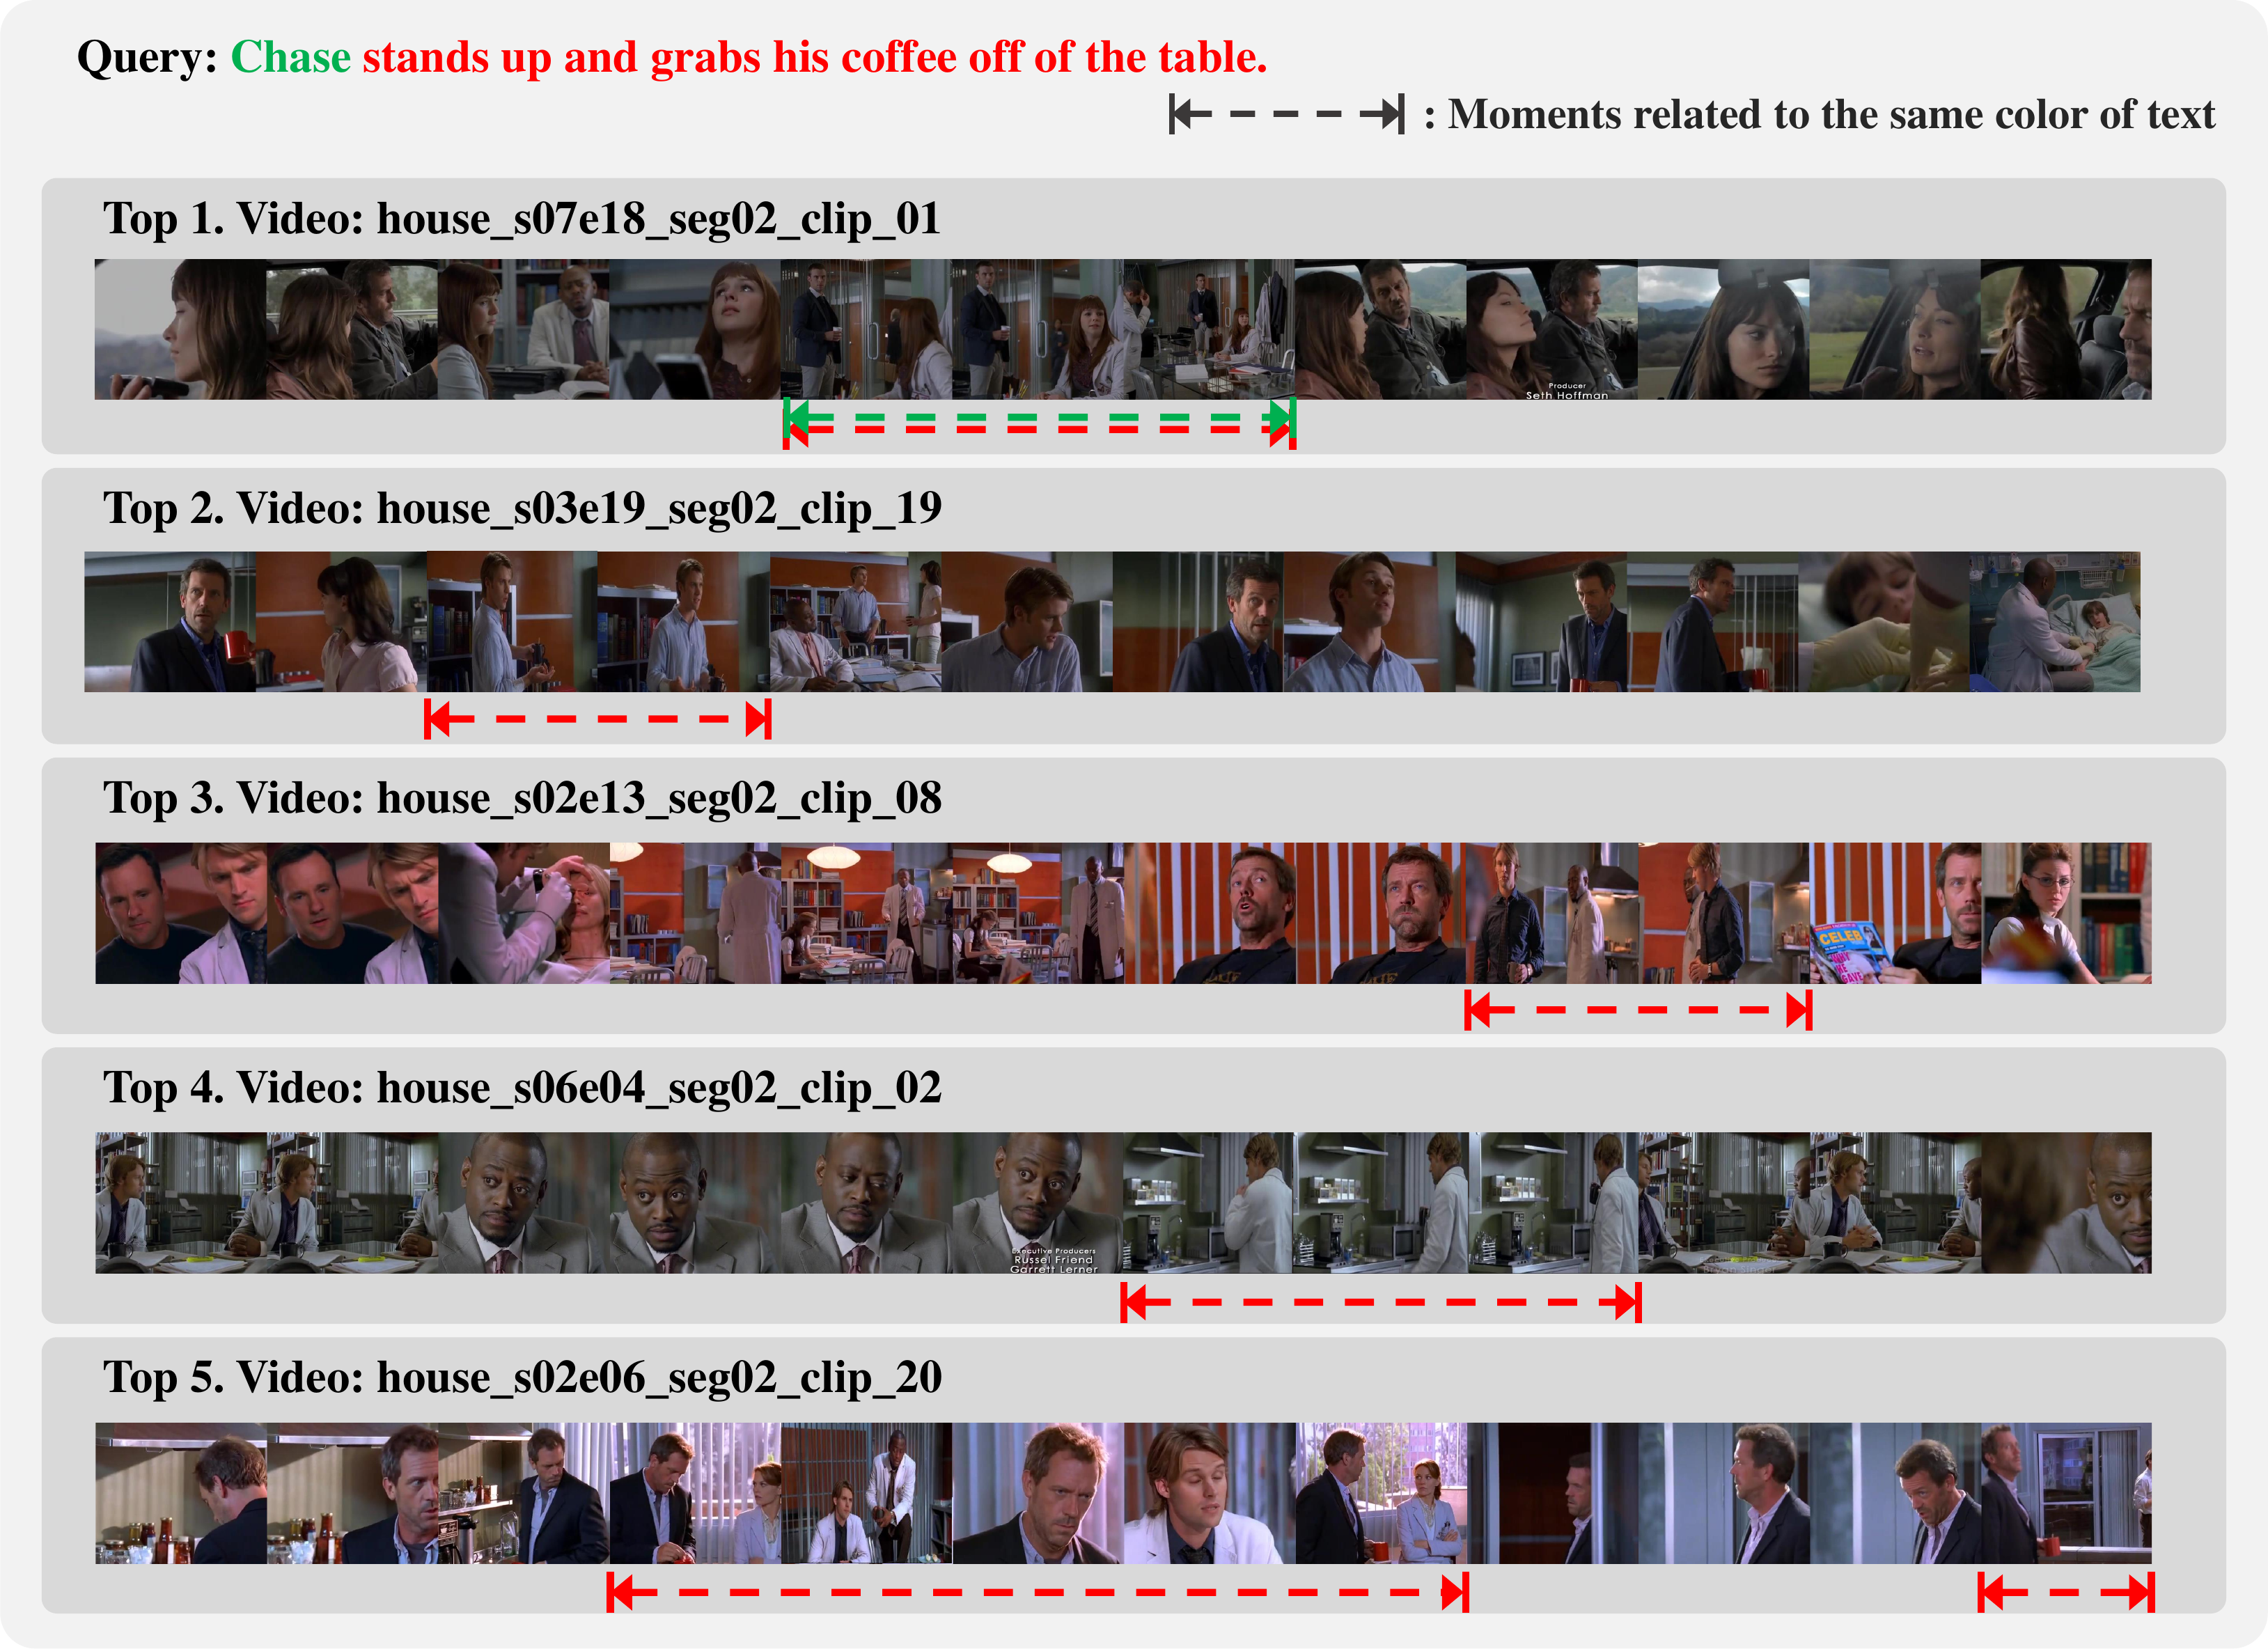}
    \includegraphics[width=0.9\textwidth]{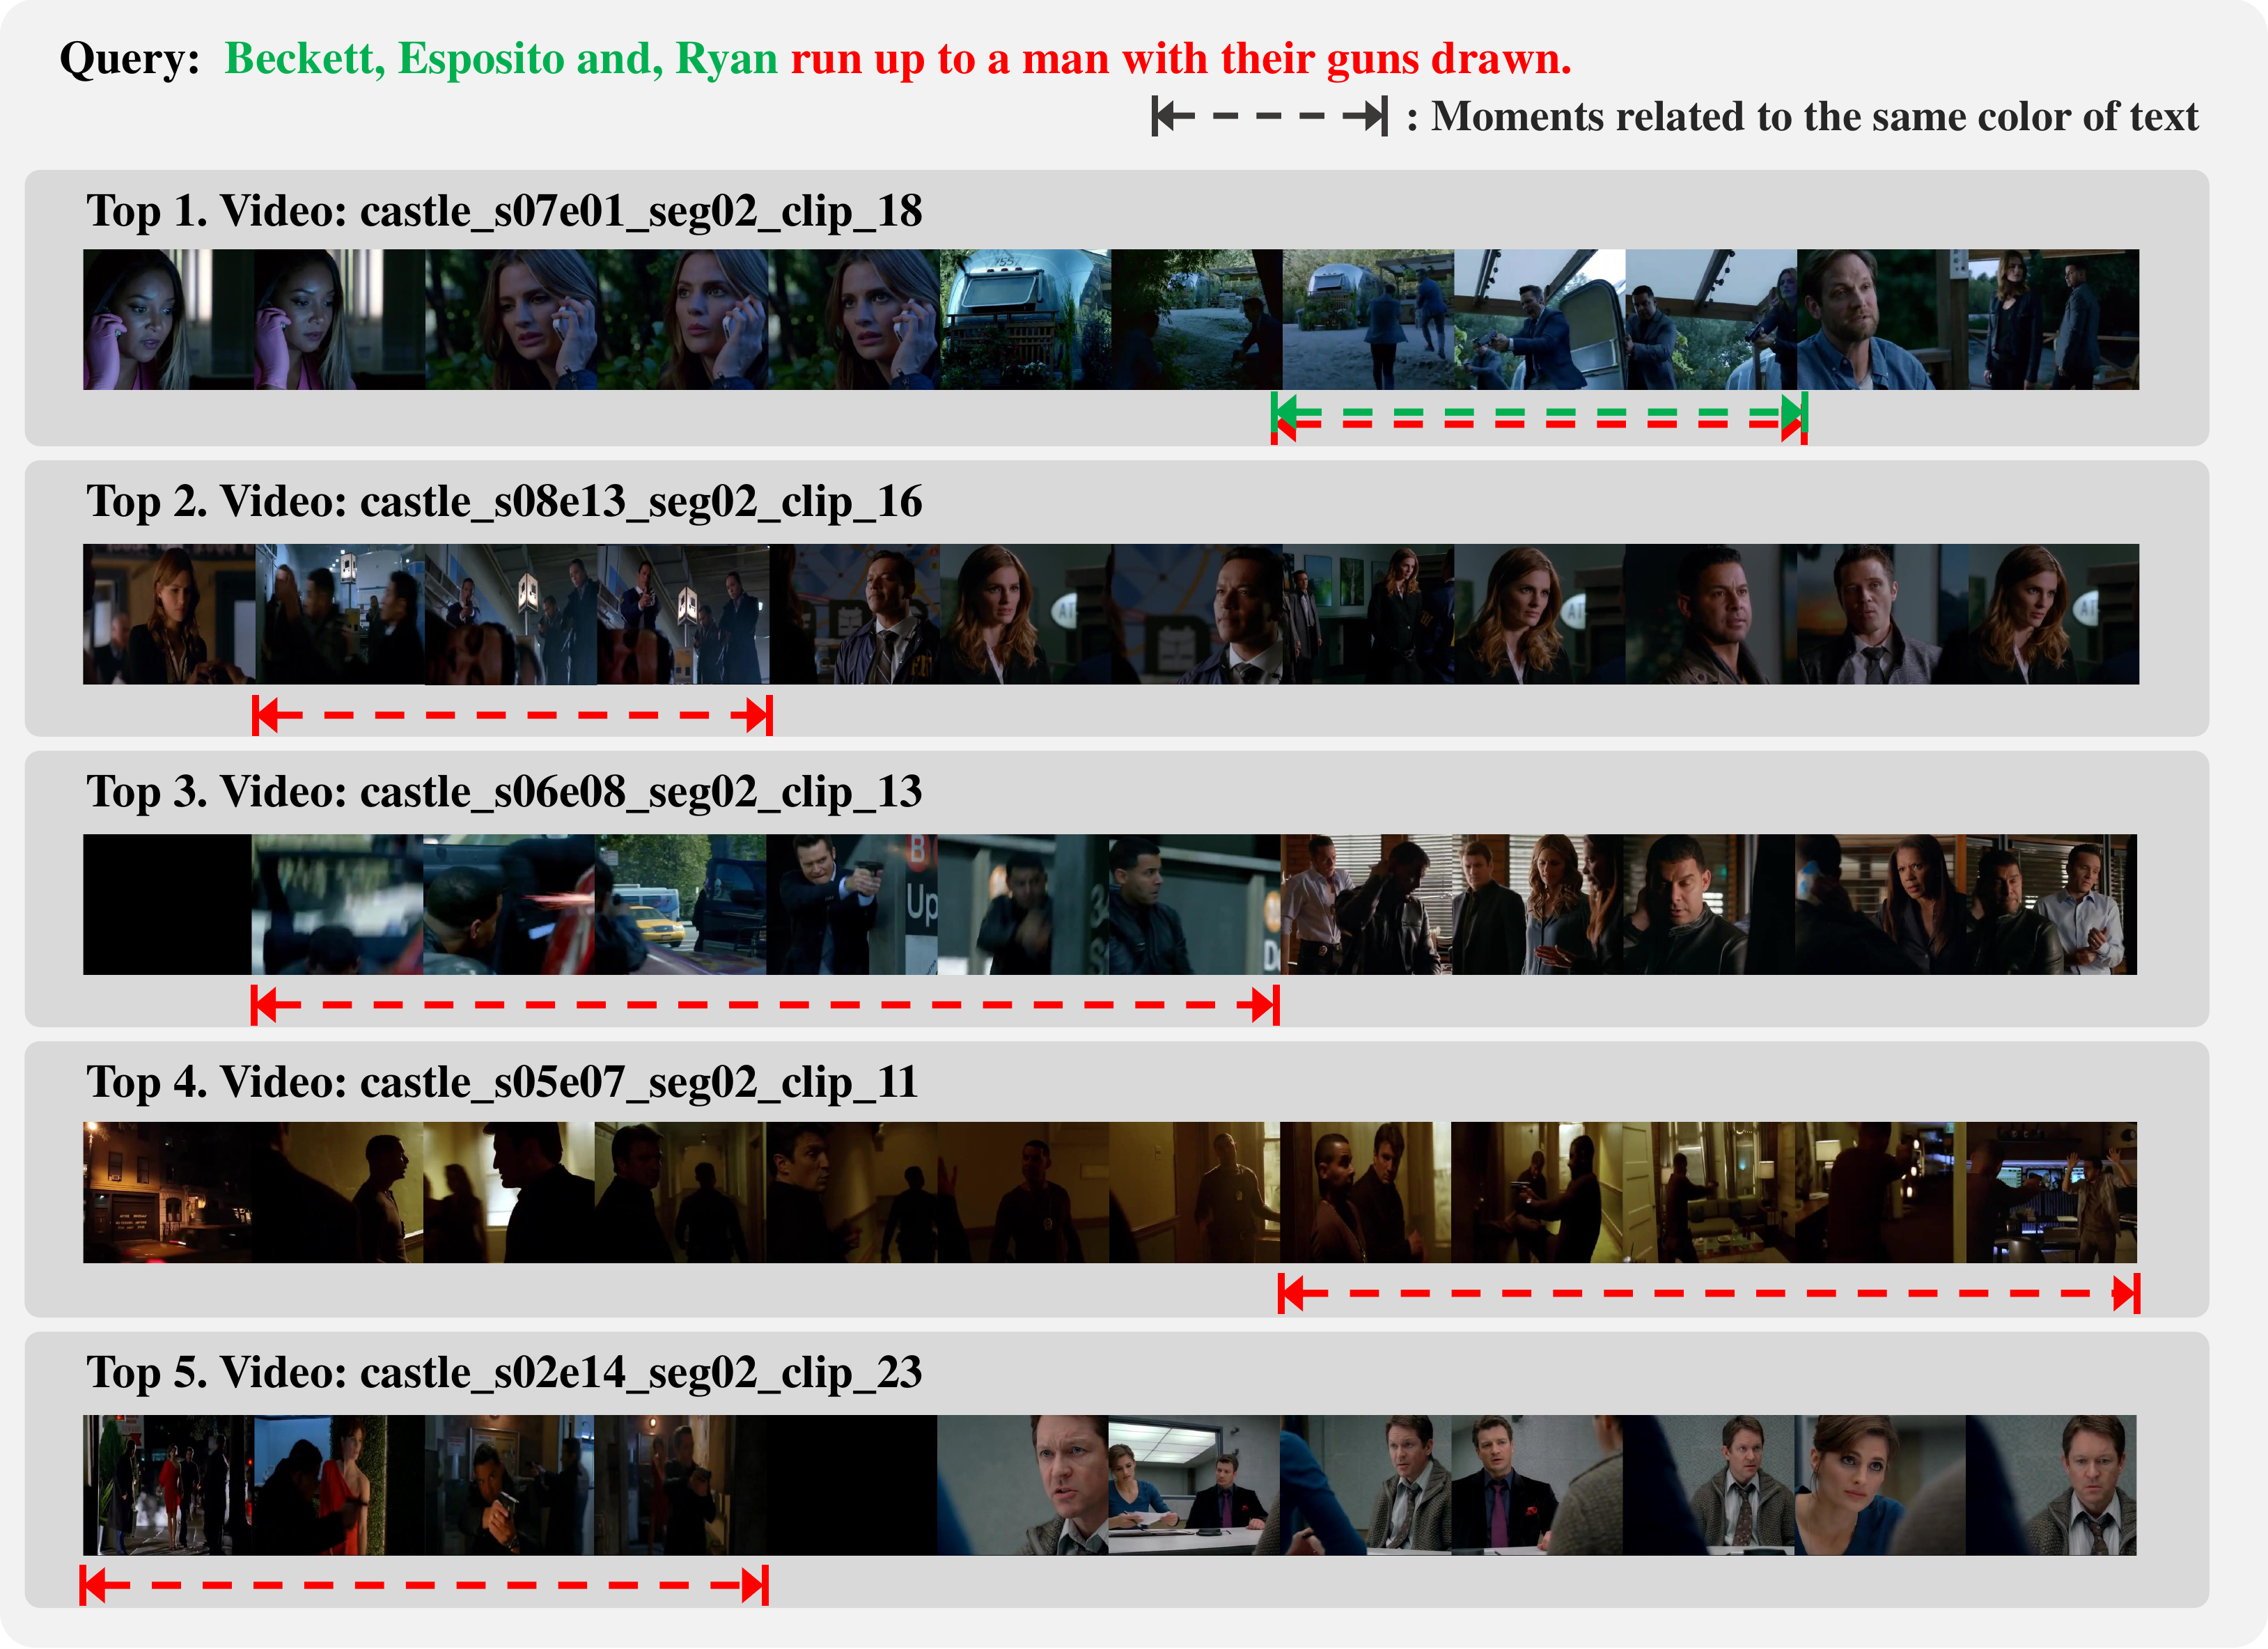}
    % \vspace{-0.3cm}
    \caption{Top-5 recall results on TVR dataset. 
    Each event in the query is colored in different colors while the corresponding moments are marked with a dotted line in the same color if the context exists in the video.
    }
    \label{fig:top5_qualitative}
    % \vspace{-0.5cm}
\end{figure*}
\begin{figure*}[t!]
    \centering
    % \vspace{-0.3cm}
    \includegraphics[width=0.88\textwidth]{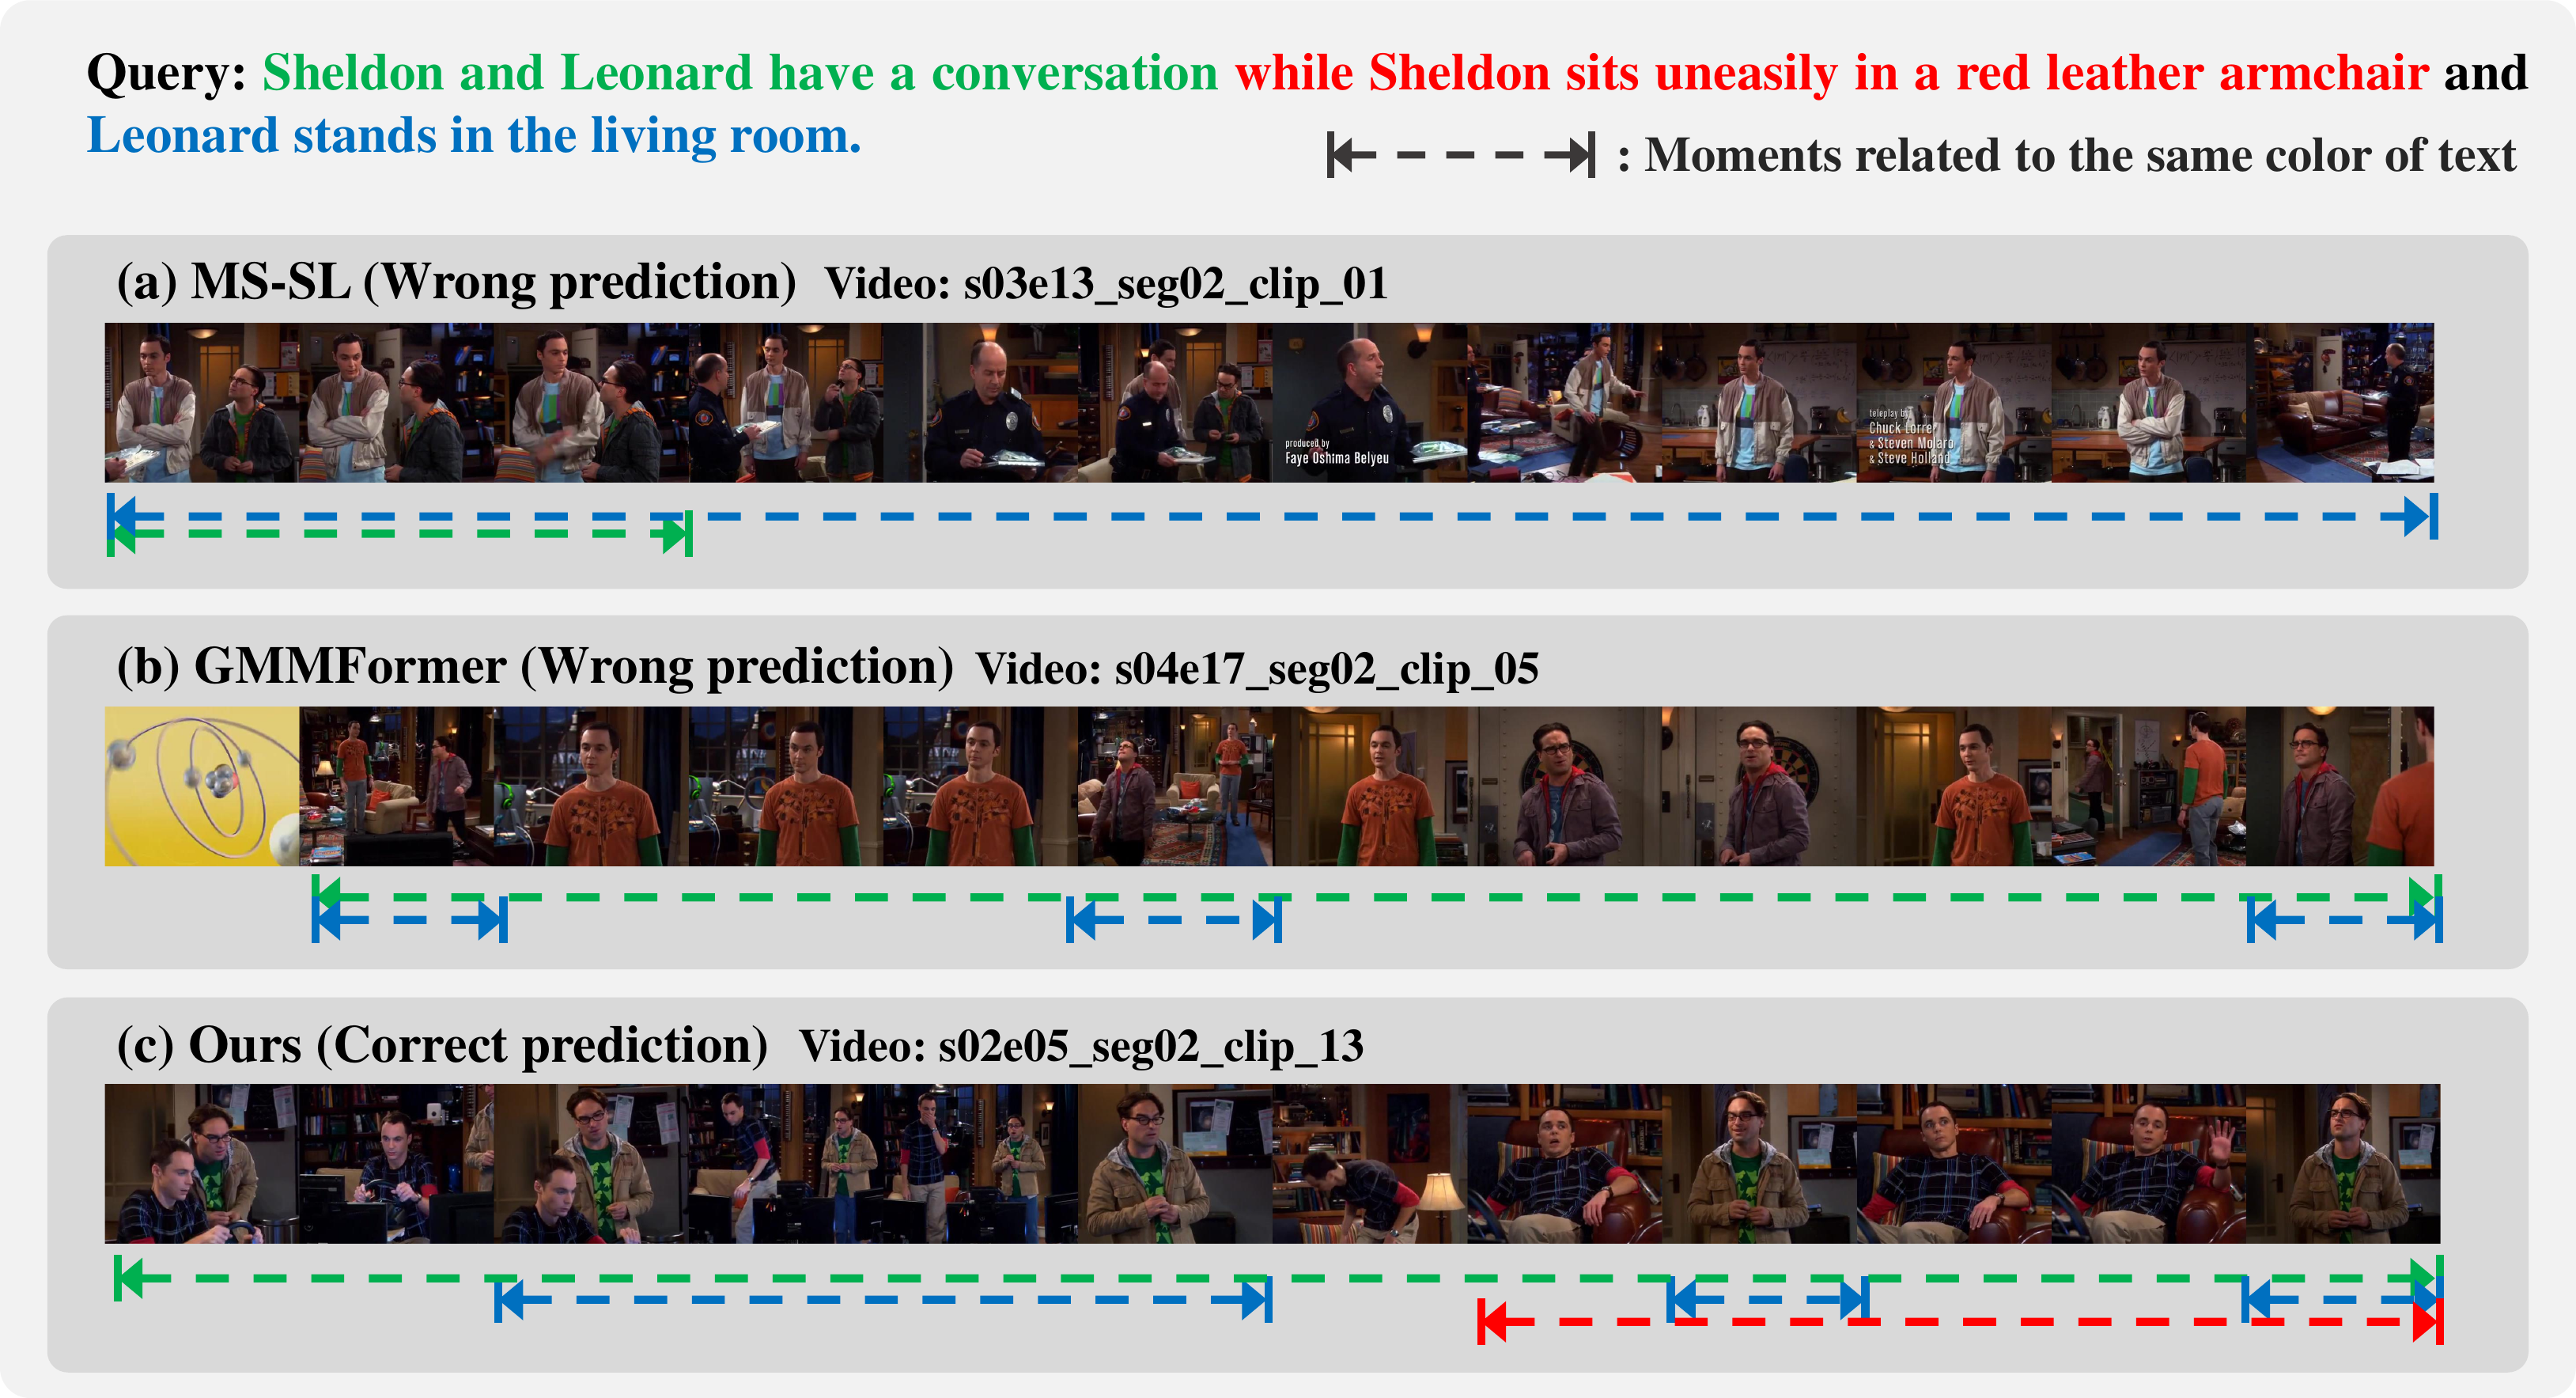}
    \includegraphics[width=0.88\textwidth]{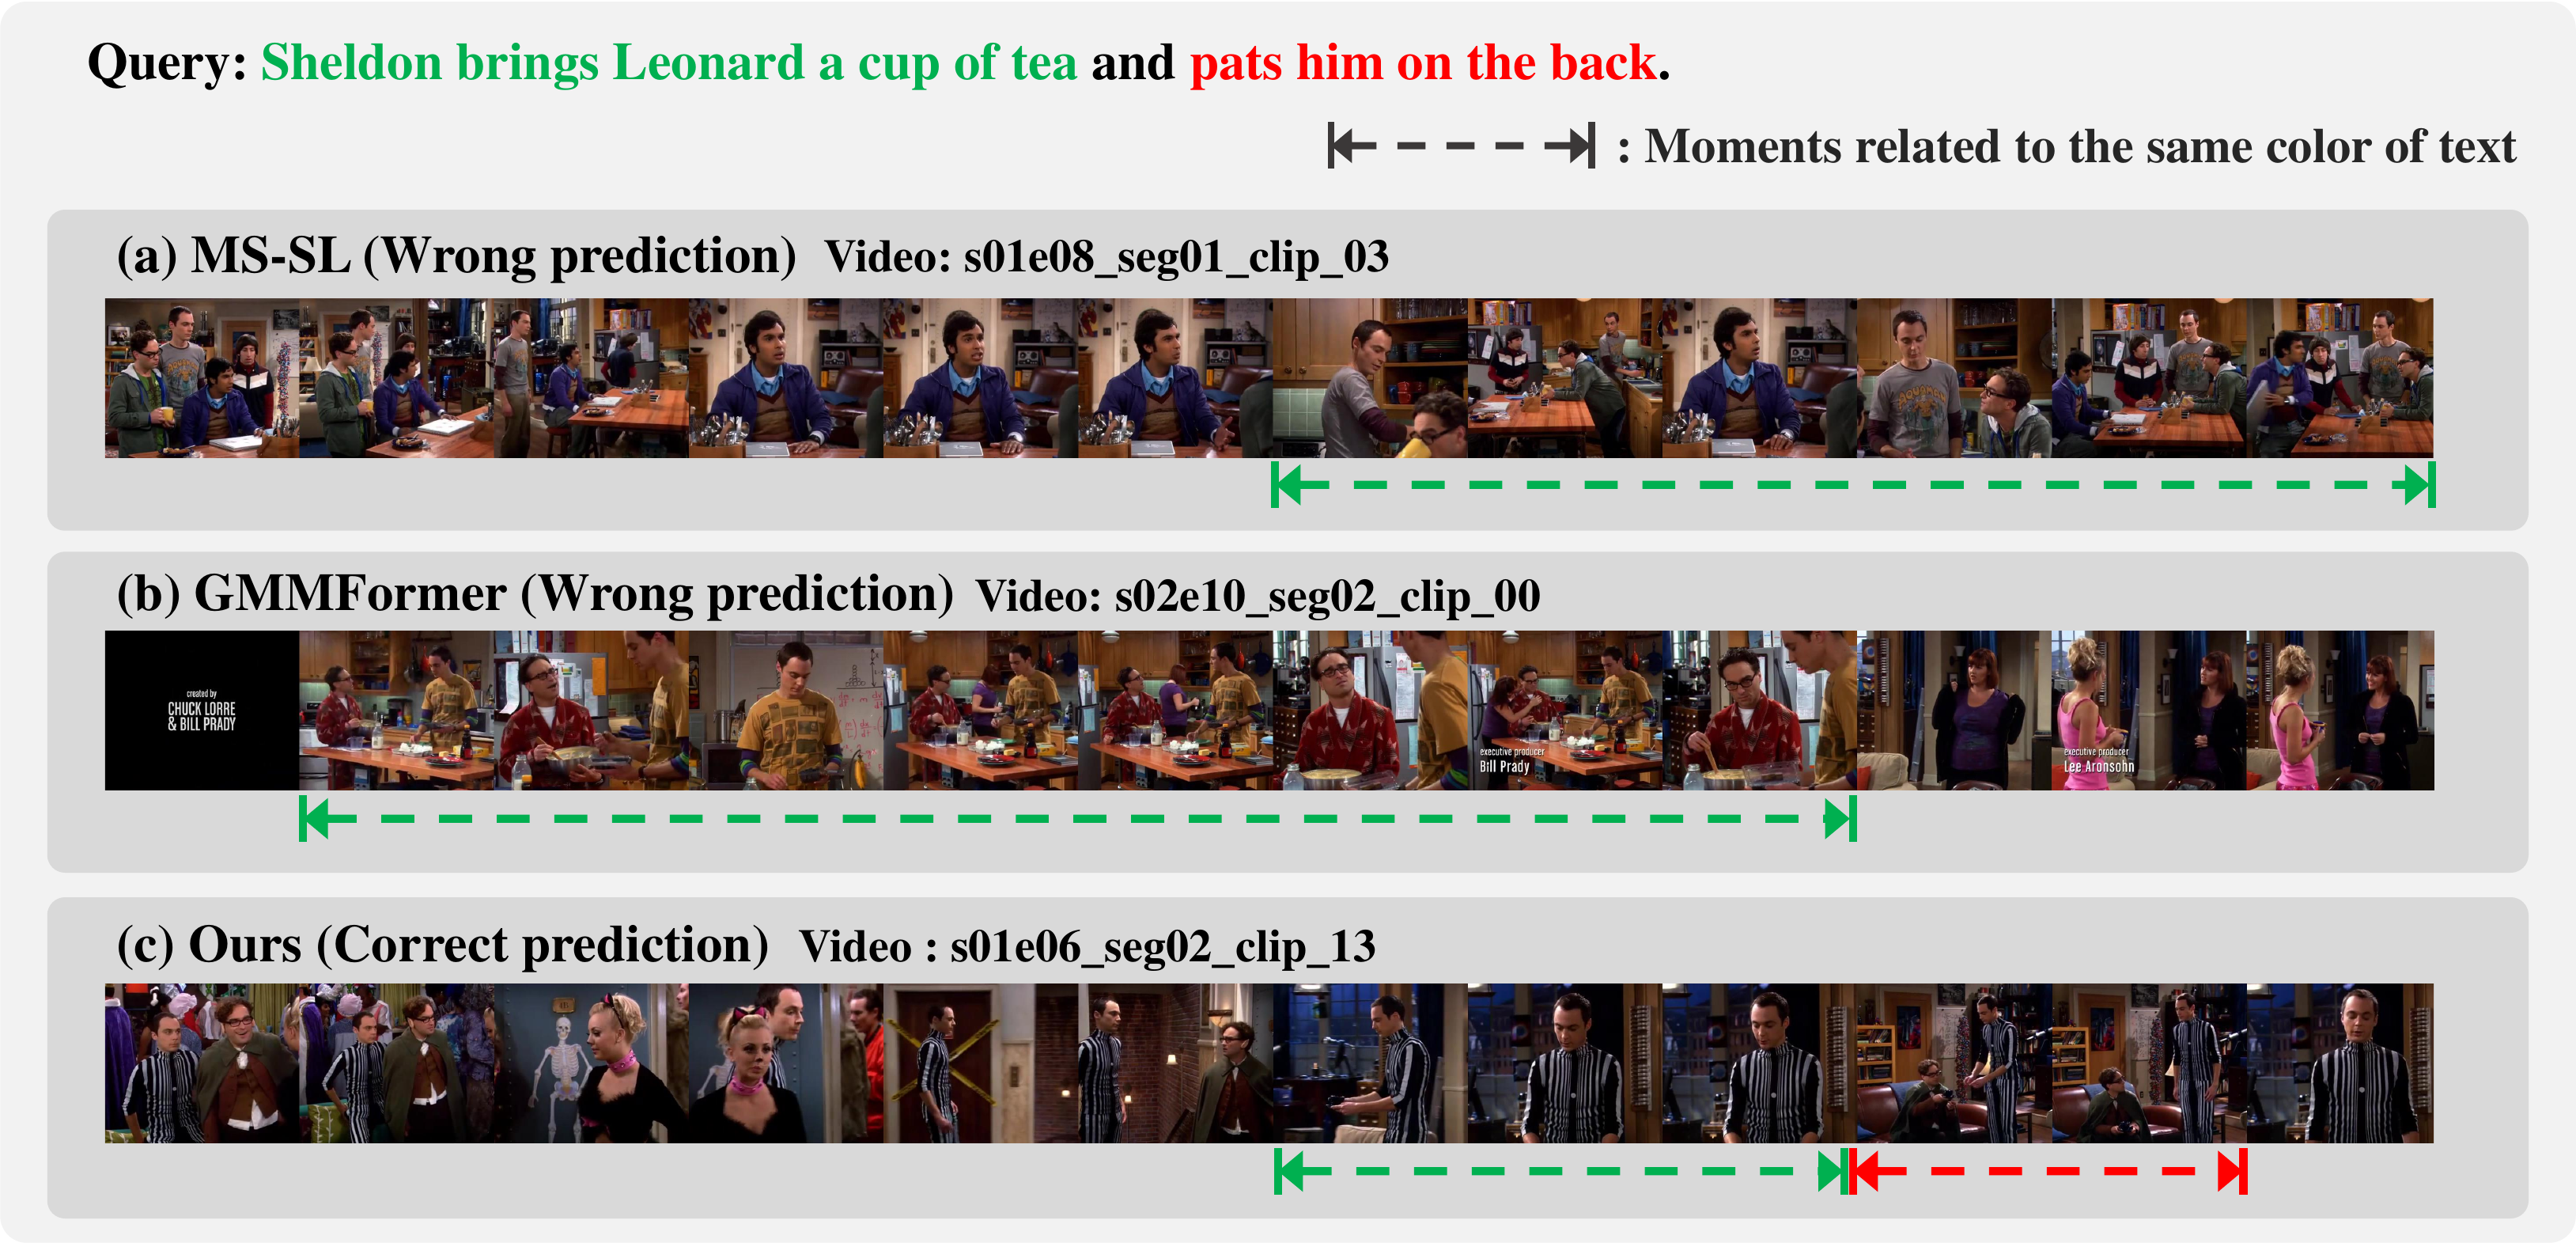}
    \includegraphics[width=0.88\textwidth]{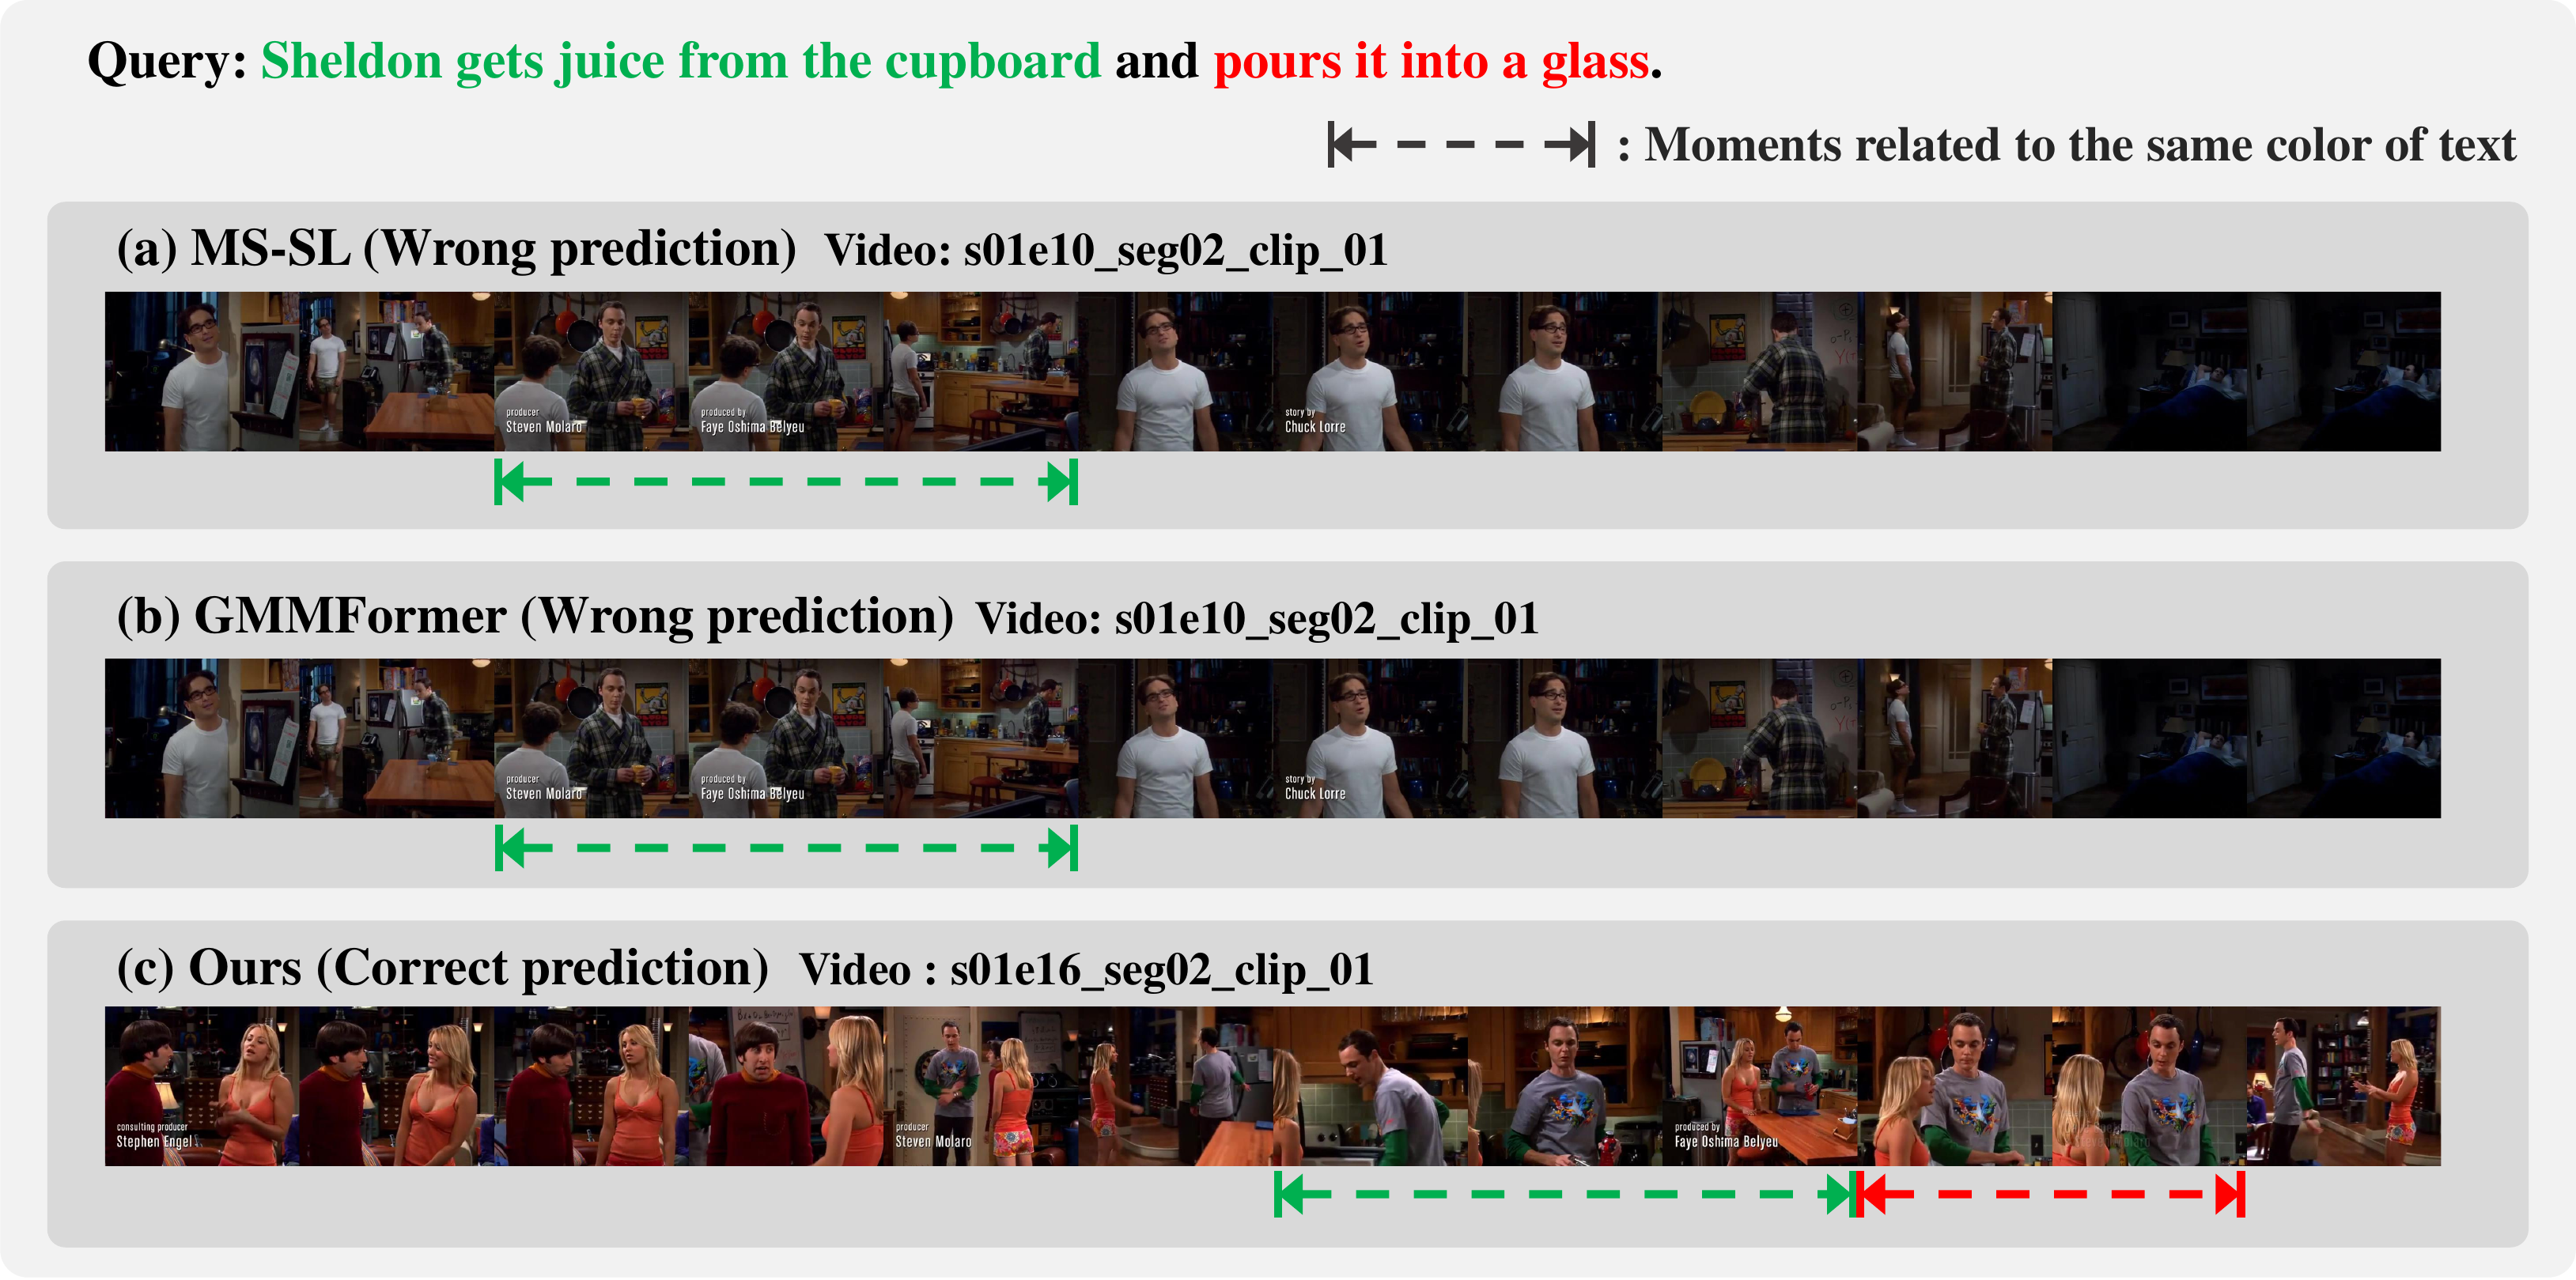}
    % \vspace{-0.3cm}
    \caption{Qualitative results on TVR dataset. 
    Each event in the query is colored in different colors while the corresponding moments are marked with a dotted line in the same color if the context exists in the video.
    }
    \label{fig:more_qualitative}
    % \vspace{-0.5cm}
\end{figure*}

\section{Additional Qualitative Results}
\label{sec:sup_qualitative}
\noindent\textbf{Top-ranked Predictions.}
We describe how our prototypical learning framework understands the given context with the five similar videos in Fig.~\ref{fig:top5_qualitative}.
We find consistent results among the top-5 retrieved videos that they share a similar concept with the text query. 
Specifically, in the first example, the high-ranked retrieved videos accurately depict the context described in the text query, with the exception that only the subject performing the action differs.

\noindent\textbf{Additional Qualitative Results.} 
Additional qualitative results along with the results from the baselines are depicted in Fig.~\ref{fig:more_qualitative}.
While the baselines struggle with searching the video with the precise contexts, our proposed method shows its strength in understanding sequential events.
For example, retrieved videos of the baselines only include the partial concept; in the first example, videos only with two simultaneous events are retrieved, and retrieved videos only include the partial event of getting the juice in the second example.
